# Supplementary material for: Compression stiffening of fibrous networks with stiff inclusions
Source: arXiv:2002.07220 ancillary file (2020-07-05)
Supplement: Supplementary file 1 [file SI_Appendix.pdf]

## Supplemental Information:
## Compression stiffening of fibrous networks with stiff inclusions

Jordan Shivers,[1,2] Jingchen Feng,[2] Anne S. G. van Oosten,[3]
Herbert Levine,[2,4] Paul Janmey,[3] and Fred C. MacKintosh[1,2,5]

[1]*Department of Chemical and Biomolecular Engineering, Rice University, Houston, TX 77005*
[2]*Center for Theoretical Biological Physics, Rice University, Houston, TX 77030*
[3]*Institute for Medicine and Engineering, University of Pennsylvania, Philadelphia, PA 19104*
[4]*Department of Physics and Department of Bioengineering, Northeastern University, Boston, MA 02115*
[5]*Departments of Chemistry and Physics & Astronomy, Rice University, Houston, TX 77005*

**Contents**

I. Predicting the required compression for contact percolation and jamming 1

II. Rope model 2

III. Fiber network simulations 6
A. Underlying random networks 6
1. 2D 6
2. 3D 6
B. Networks with bound inclusions 6
C. Disconnected inclusions 14

References 14

### I. Predicting the required compression for contact percolation and jamming

Consider a parallel-plate rheometer containing a gel sample occupying initial total volume $V = V_0$. The gel consists of a polymer network containing randomly distributed, rigid spherical inclusions with initial volume fraction $\phi_0$. The polymer volume fraction is negligible, and an incompressible buffer fluid fills the remaining sample volume. Assuming that the inclusions are rigid and that the network and inclusions are mechanically constrained to remain within the initial sample volume, changes in $V$ amount to fluid flow into or out of the sample. Under uniaxial strain $\varepsilon$ with zero lateral strain, the total volume of the sample becomes

$V = (1 + \varepsilon)V_0$. Note that compression corresponds to $\varepsilon < 0$. As the volume occupied by the inclusions ($\phi_0 V_0$) remains constant, the strain-dependent inclusion volume fraction is $\phi = \phi_0/(1 + \varepsilon)$. Prior work has shown that contact percolation in radially bidisperse spheres with short-range attractive interactions occurs at a particle volume fraction of $\phi_p = 0.214$ in 3D and $\phi_p \approx 0.558$ in 2D [1], under effective bulk compression. Assuming that the volume fraction for contact percolation is protocol independent (which may not be true), then for a system with initial volume fraction $\phi_0$, we can estimate the uniaxial strain required for contact percolation as $\varepsilon_p = \phi_0/\phi_p - 1$. Jamming likewise occurs at a specific particle volume fraction $\phi_j$ (for bidisperse disks in 2D, $\phi_j \approx 0.84$, and for spheres in 3D, $\phi_j \approx 0.64$ [2]). If we again assume that the jamming volume fraction is the same for bulk compression as for uniaxial compression, then for a given $\phi_0$, we can estimate the uniaxial strain required for jamming is $\varepsilon_j = \phi_0/\phi_j - 1$. As we show in the main text and in Fig. S1, this estimate agrees with our simulations.

## II. Rope model

In Fig. S1, we show the complementary figure to Fig. 2 in the main text for the 2D rope model, using radially bidisperse disks. We note that, for an intermediate range of initial particle area fractions, stretching-dominated stress propagation in the $\lambda = 1$ limit occurs at lower levels of applied compression than predicted for contact percolation ($\varepsilon_p = \phi_0/\phi_p - 1$), whereas this is not observed in our 3D results. In Fig. S2, we sketch examples of systems in which stretching-dominated stress propagation for $\lambda = 1$ occurs concurrently with contact percolation (Fig. S2a) and before contact percolation (Fig. S2b). In Fig. S3a, we plot the critical compressive strain $\varepsilon_c$ for stretching-dominated stress propagation in the 2D rope model as a function of the slack extension of the rope-like springs, $\lambda_c - 1$, for varying $\phi_0$. In Fig. S3b, we plot the same data for the 3D rope model, as described in the main text. To predict the critical compressive strain for stretching-dominated stress propagation in a system with inclusion volume fraction $\phi_0$ and network connectivity $z$, we interpolate between the measured points to find $\varepsilon_c(\phi_0, \lambda_c = 1 + \varepsilon_c(\phi = 0, z))$, where $\varepsilon_c(\phi = 0, z)$ is the critical extensional strain for an inclusion-free network of connectivity $z$.

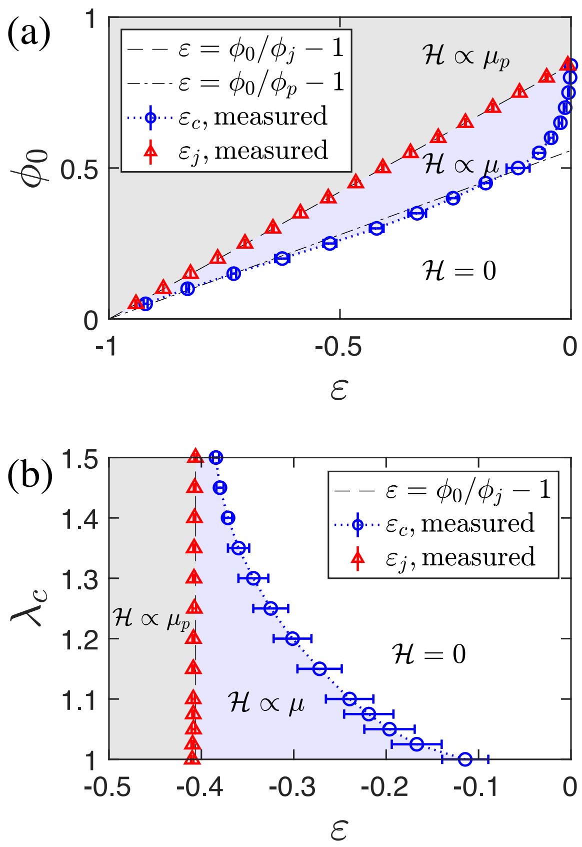


FIG. S1. (a) Mechanical phase diagram for compressed systems of $N = 900$ radially bidisperse, repulsive disks, in which nearest neighbors (by Delaunay triangulation) are connected by rope-like springs, as a function of uniaxial strain $\varepsilon$ and initial volume fraction $\phi_0$. Here, $\mu = 10^{-5}$, $\mu_p = 1$, and the rope-like springs have slack extension $\lambda_c = 1$. The blue circles correspond to the critical strain for the onset of stretching-dominated stress propagation, $\varepsilon_c$, and the red triangles correspond to the onset of jamming, $\varepsilon_j$. The dashed black line corresponds to the predicted applied strain required for jamming of a system with initial volume fraction $\phi_0$, $\varepsilon_j = \phi_0/\phi_j - 1$, in which $\phi_j = 0.84$. The white region corresponds to the floppy regime ($\mathcal{H} = 0$, blue corresponds to the stretching-dominated regime ($\mathcal{H} \propto \mu$), and gray corresponds to the jammed regime ($\mathcal{H} \propto \mu_p$). (b) Mechanical phase diagram for volume fraction $\phi_0 = 0.5$ as a function of applied uniaxial strain $\varepsilon$ and slack extension of rope-like springs, $\lambda_c$. Error bars in both panels correspond to $\pm 1$ standard deviation.

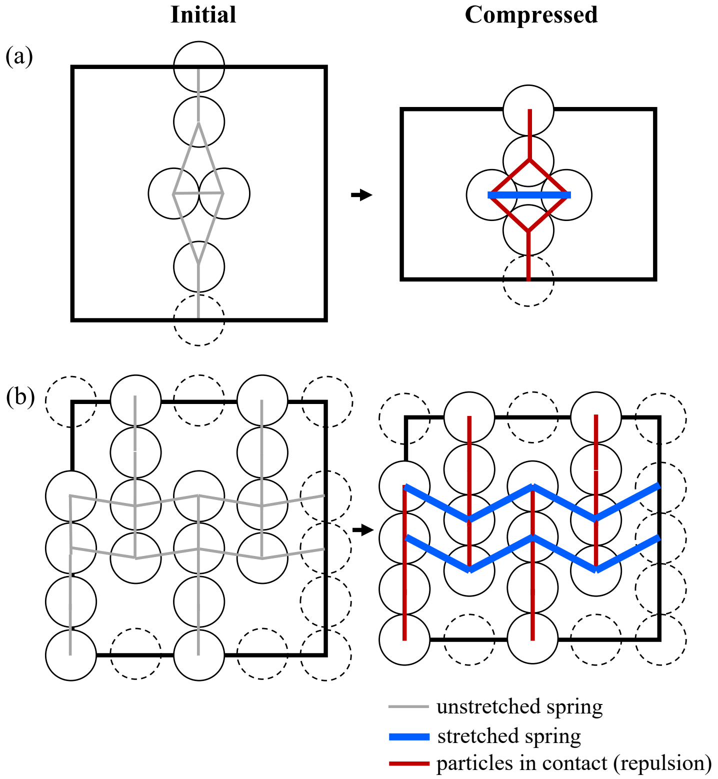


FIG. S2. Illustrations of periodic assemblies of particles connected by rope-like springs in which, under applied uniaxial compression, stretching-dominated stress propagation occurs (a) concurrent with contact percolation and (b) prior to contact percolation.

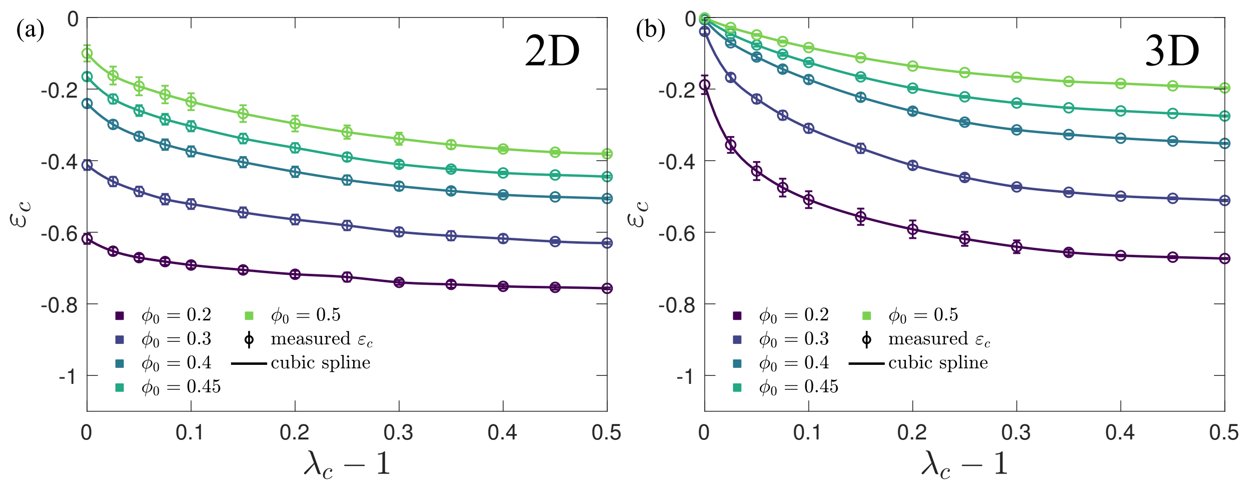


FIG. S3. Measured critical strain values for compression-driven, stretching-dominated stress propagation in (a) the 2D rope model for systems with $N = 900$ radially bidisperse disks and (b) the 3D rope model for systems with $N = 1000$ radially monodisperse spheres, with varying initial volume fraction $\phi_0$, as a function of the slack extension of the rope-like springs, $\lambda_c$. Circles represent measured values and solid lines represent cubic spline fits used to interpolate between measured points. We use this plot to empirically predict the critical strain for compression-driven stiffening in simulated particle-network composites in which the interstitial network has a known critical extensile strain.

## III. Fiber network simulations

### A. Underlying random networks

Below we describe the procedures for generating random packing-derived networks in 2D and 3D, to which we eventually insert inclusions.

#### *1. 2D*

To generate 2D packing-derived networks, we randomly place $N = L^2$ radially bidisperse disks with $r \in (r_0, 1.4r_0)$ in a periodic square unit cell of side length $L$ and incrementally increase $r_0$ from 0, allowing the system to relax at each step, until the average connectivity of the contact network (joining overlapping disks) exceeds 5.5. We use a ratio of radii of 1.4 to prevent the particles from developing crystalline order [3]. We then selectively remove bonds from the most highly connected pairs of nodes, in order to minimize spatial heterogeneity in the connectivity [4], until the desired average connectivity $z$ is reached. During the dilution procedure, dangling ends are also removed.

#### *2. 3D*

To generate 3D packing-derived networks, we randomly place $N = L^3$ spheres of radius $r_0$ in a periodic cubic unit cell of side length $L$ and incrementally increase $r_0$ from 0, allowing the system to relax at each step, until the average connectivity of the contact network (joining overlapping disks) exceeds 8. We then selectively remove bonds from the most highly connected pairs of nodes, in order to minimize spatial heterogeneity in the connectivity [4], until the desired average connectivity $z$ is reached. During the dilution procedure, dangling ends are also removed. In Fig. S4, we show a 3D network with $L = 15$ and $z = 4$ prior to the addition of inclusions.

### B. Networks with bound inclusions

After the underlying fiber network is generated, non-intersecting inclusions (disks in 2D and spheres in 3D) are randomly placed until the desired inclusion volume fraction is reached. Bonds that intersect with the surface of a placed inclusion are connected to the inclusion surface, at the intersection point, by a freely rotating joint, and all bond segments within the inclusion boundary are removed. Each inclusion behaves as a rigid $d$-dimensional body with $d$ translational and $x$ rotational degrees of freedom ($x = 1$ for $d = 2$, and

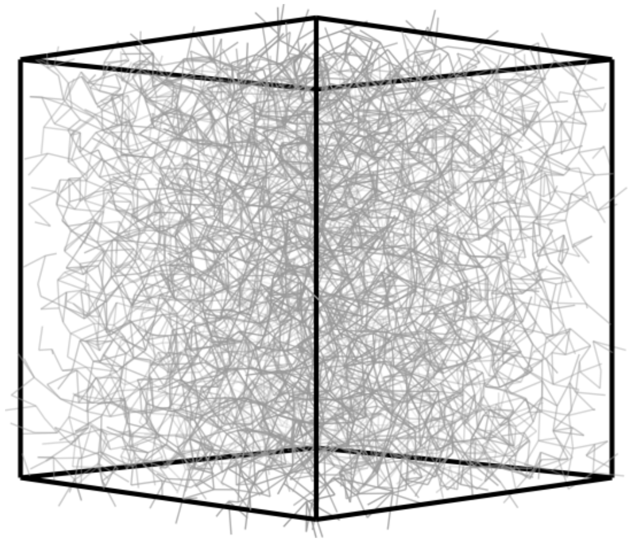

FIG. S4. Periodic network made up of $15^3$ nodes with average connectivity $z = 4$.

$x = 3$ for $d = 3$), such that all of the boundary connections translate and rotate rigidly with the inclusion. In Fig. S5, we show images of the resulting networks, containing inclusions, in 2 and 3 dimensions. In 2D, we use radially bidisperse circular inclusions, with a ratio of radii of 1.4, in which half of the inclusions have the larger radius $R = 4$.

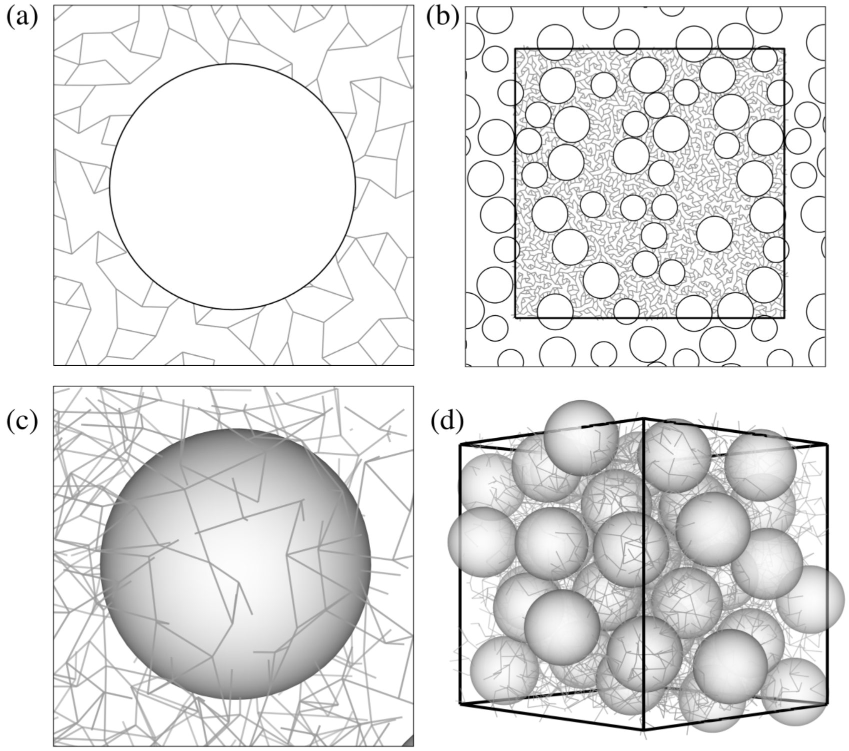


FIG. S5. (a) Single inclusion of radius $R = 4$ in a 2D packing-derived network with $z = 3$. Bonds that intersect with the inclusion boundary are rigidly connected to the boundary, at the point of intersection, by a freely rotating joint. One-sided repulsive interactions act both between inclusions whose boundaries overlap and between inclusion boundaries and network nodes. (b) Example of an initial configuration of a packing-derived network with $z = 3$ and radially bidisperse inclusions, with area fraction $\phi_0 = 0.4$. (b) Single inclusion of radius $R = 2$ in a 3D packing-derived network with $z = 4$. (b) Example of an initial configuration of a 3D packing-derived network with $z = 4$ and inclusion volume fraction $\phi_0 = 0.4$.

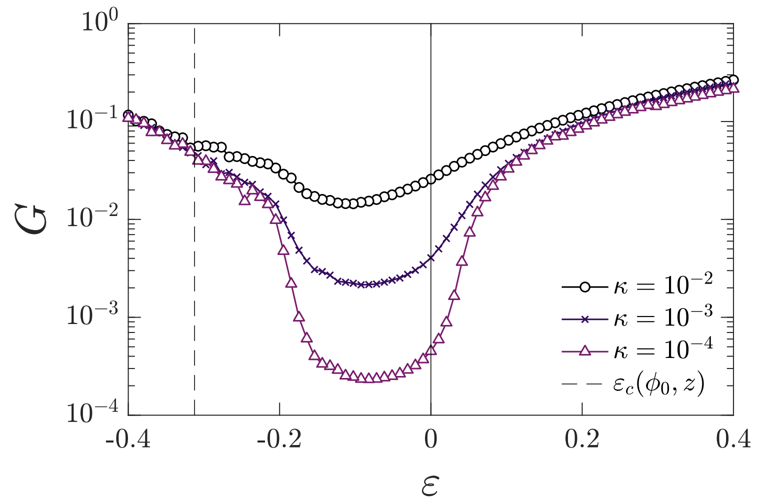


FIG. S6. Shear modulus $G$ for 3D packing-derived networks with $\phi = 0.4$, $z = 4$, varying bond-bending modulus $\kappa$ and constant stretching modulus $\mu = 1$. These systems undergo a transition from a regime in which $G \propto \kappa$ at low levels of applied compression to one in which $G \propto \mu$ (independent of $\kappa$) at higher compression levels.

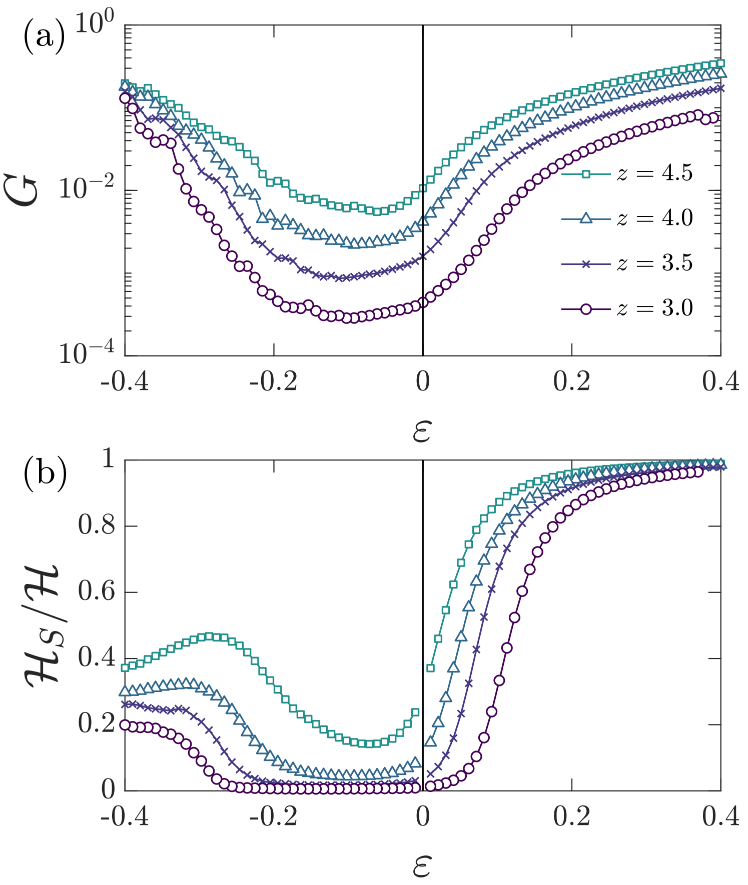


FIG. S7. (a) Shear modulus $G$ and (b) stretching energy fraction $\mathcal{H}_S/\mathcal{H}$ as a function of applied uniaxial strain $\varepsilon$ for 3D packing-derived networks with $\phi_0 = 0.4$, $\kappa = 10^{-3}$, and varying average connectivity $z$. Under both compression and extension, increasing $z$ leads to a decrease in the magnitude of strain required the onset of the stiff stretching-dominated regime.

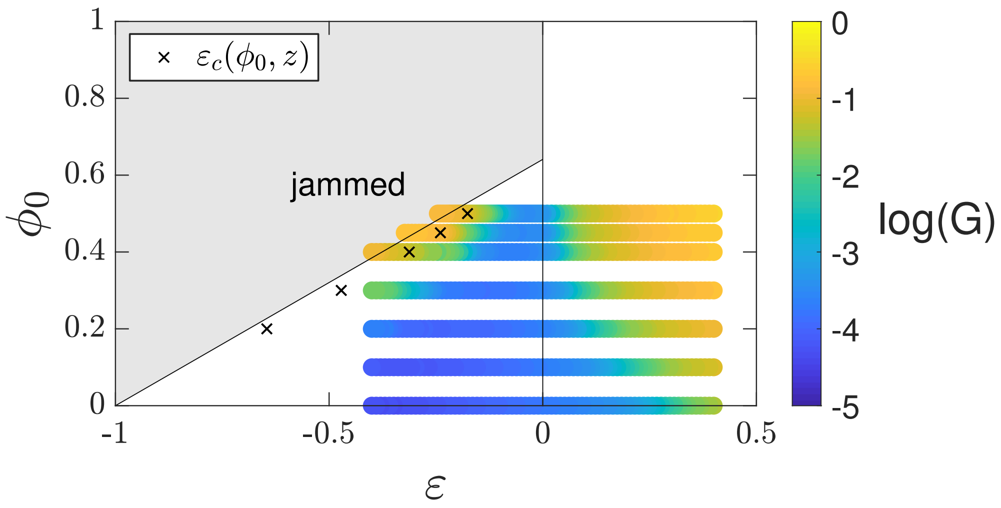


FIG. S8. Data from Fig. 3a in the main text:. Phase diagram depicting the shear modulus for 3D packing-derived networks with $z = 4$ and $\kappa = 10^{-4}$ as a function of inclusion volume fraction $\phi_0$. Each $x$ denotes the predicted critical compressive strain for stretching-dominated stress propagation for the rope model with volume fraction $\phi_0$, using an appropriate value of the slack extension $\lambda_c$ to account for the extensional critical strain $\varepsilon_{c,ext}$ of 3D packing-derived networks with $z = 4$ , i.e. $\lambda_c = 1 + \varepsilon_{c,ext}(z = 4) \approx 1.3$.

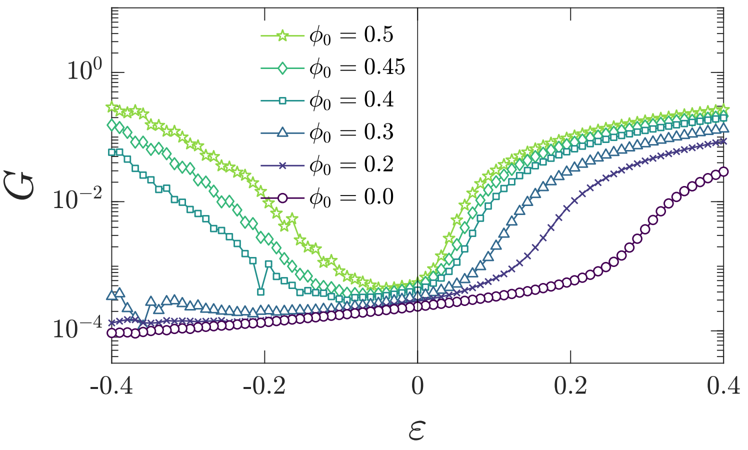


FIG. S9. (a) Shear modulus $G$ as a function of applied uniaxial compression $\varepsilon$ for 2D packing-derived networks with $z = 3$, $\kappa = 10^{-4}$, and varying initial inclusion area fraction $\phi_0$.

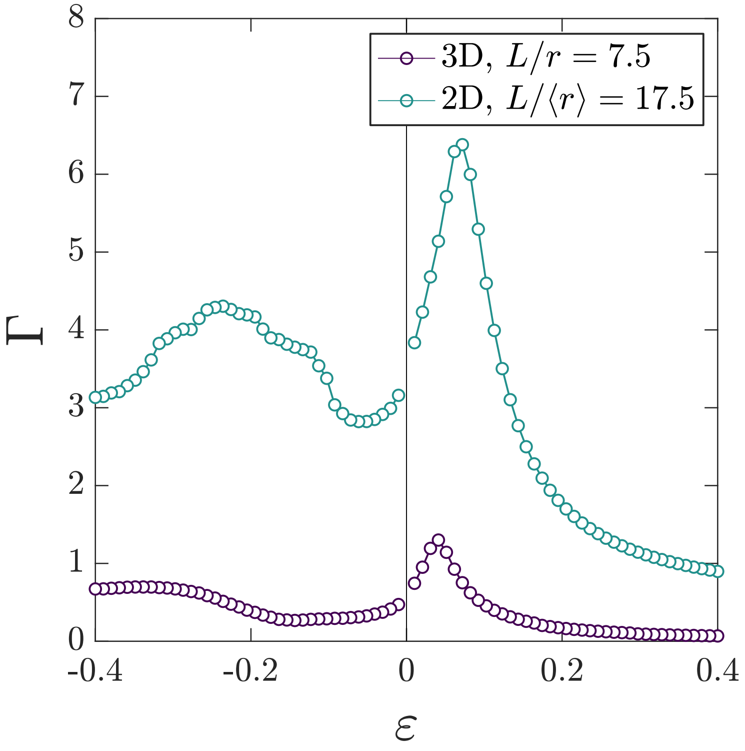


FIG. S10. Comparison of the strain-dependent inclusion nonaffinity between 2D and 3D packing-derived networks containing inclusions with $\kappa = 10^{-4}$ and volume fraction (area fraction in 2D) $\phi_0$. The 3D data correspond to $z = 4$, $L = 15$, and $r = 2$, and the 2D data correspond to $z = 3$, $L = 60$, and average inclusion radius $\langle r\rangle = 3.43$ (we use radially bidisperse inclusions in 2D; half the inclusions are of radius 4 and half $4/1.4$). Given that the ratio of the system size to the inclusion radius is larger in our 2D simulations than in our 3D simulations, it is unsurprising that the 2D systems exhibit more heterogeneous inclusion deformation. Future work will be necessary to explore the system size dependence of Γ in 2D and 3D.

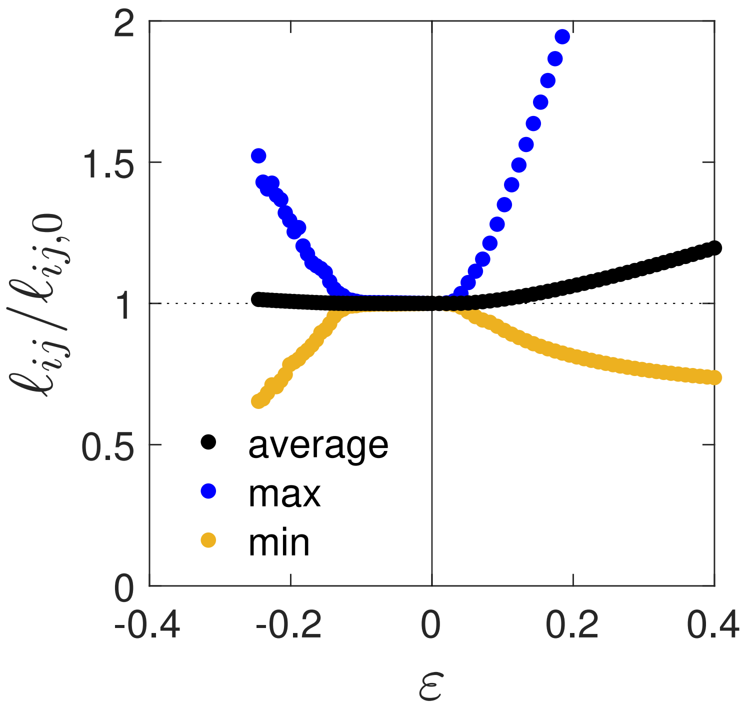


FIG. S11. Average, minimum, and maximum bond change in bond length for a 3D packing-derived network with $\phi_0 = 0.5$, $z = 4$, and $\kappa = 10^{-4}$. Under compression, we find that the maximum extension of any individual bond does not exceed roughly 50%, even as the system approaches the jamming point. For systems with highly extensible bonds, such as fibrin (which can tolerate extensional strains of over 200% [5]), we can thus expect compression-driven stiffening to occur without stretching-induced bond rupture.

### C. Disconnected inclusions

To test whether bonds between the inclusions and surrounding network are necessary for compression-stiffening, we also consider 2D systems in which the locations of the (radially bidisperse) inclusions are chosen as discussed above, but all bonds are cut within radius $r_{final}/2$ of each inclusion center and then the repulsive inclusion is swollen from radius 0 to $r_{final}$ (in which $r_{final} = R$ or $R/1.4$). In this case, each inclusion interacts with the surrounding network only through repulsive interactions. Parameters are otherwise chosen to be the same as for the 2D data presented in Fig. S9. As shown in Fig. S12a, the initial inclusion swelling induces prestress within the interstitial network. The corresponding shear moduli, as a function of axial strain, for such systems with varying $\phi_0$.

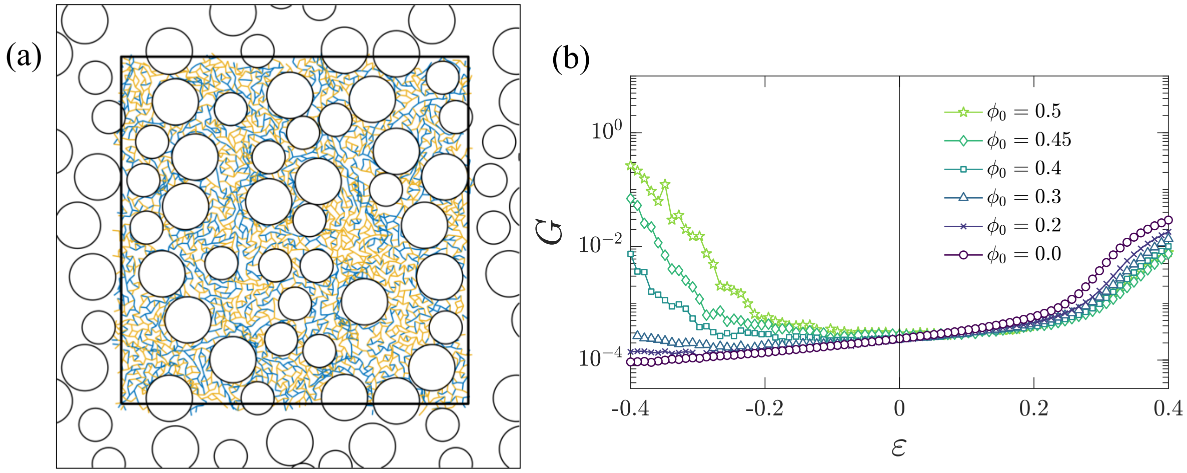


FIG. S12. (a) 2D packing-derived network with $z = 3$ and radially bidisperse inclusions with $r \in 3, 3/1.4$ and $\phi_0 = 0.4$ that are not connected to the surrounding network. Blue segments are stretched and orange segments are compressed. (b) Shear modulus $G$ as a function of applied uniaxial compression $\varepsilon$ for packing-derived networks with $z = 3$, $\kappa = 10^{-4}$, and varying initial inclusion area fraction $\phi_0$

[1] G. Lois, J. Blawzdziewicz, and C. S. O'Hern, Physical Review Letters **100**, 28001 (2008).
[2] C. S. O'Hern, S. A. Langer, A. J. Liu, and S. R. Nagel, Physical Review Letters **88**, 75507 (2002).
[3] D. J. Koeze, D. Vågberg, B. B. Tjoa, and B. P. Tighe, Europhysics Letters **113**, 54001 (2016).
[4] M. Wyart, H. Liang, A. Kabla, and L. Mahadevan, Physical Review Letters **101**, 215501 (2008).
[5] A. E. X. Brown, R. I. Litvinov, D. E. Discher, P. K. Purohit, and J. W. Weisel, Science **325**, 741 (2009).
